# Supplementary material for: Imaging of interlayer coupling in van der Waals heterostructures using a bright-field optical microscope
Source: arXiv:1612.07969 source file (2017-05-01)
Supplement: Supplementary file 1 [file SI_InterlayerCouplingImaging.pdf]

# Supporting information for: Imaging of interlayer coupling in van der Waals heterostructures using a bright-field optical microscope

Evgeny M. Alexeev,[*,†] Alessandro Catanzaro,[†] Oleksandr V. Skrypka,[†] Pramoda K. Nayak,[‡] Seongjoon Ahn,[‡] Sangyeon Pak,[¶] Juwon Lee,[¶] Jung Inn Sohn,[¶] Kostya S. Novoselov,[§] Hyeon Suk Shin,[‡] and Alexander I. Tartakovskii[*,†]

*Department of Physics and Astronomy, University of Sheffield, Sheffield S3 7RH, UK, Department of Energy Engineering and Department of Chemistry, Ulsan National Institute of Science and Technology (UNIST), 50 UNIST-gil, Ulsan 44919, Republic of Korea, Department of Engineering Science, University of Oxford, Oxford OX1 3PJ, UK, and School of Physics and Astronomy, University of Manchester, Oxford Road, Manchester M13 9PL, UK*

E-mail: e.alexeev@sheffield.ac.uk; a.tartakovskii@sheffield.ac.uk

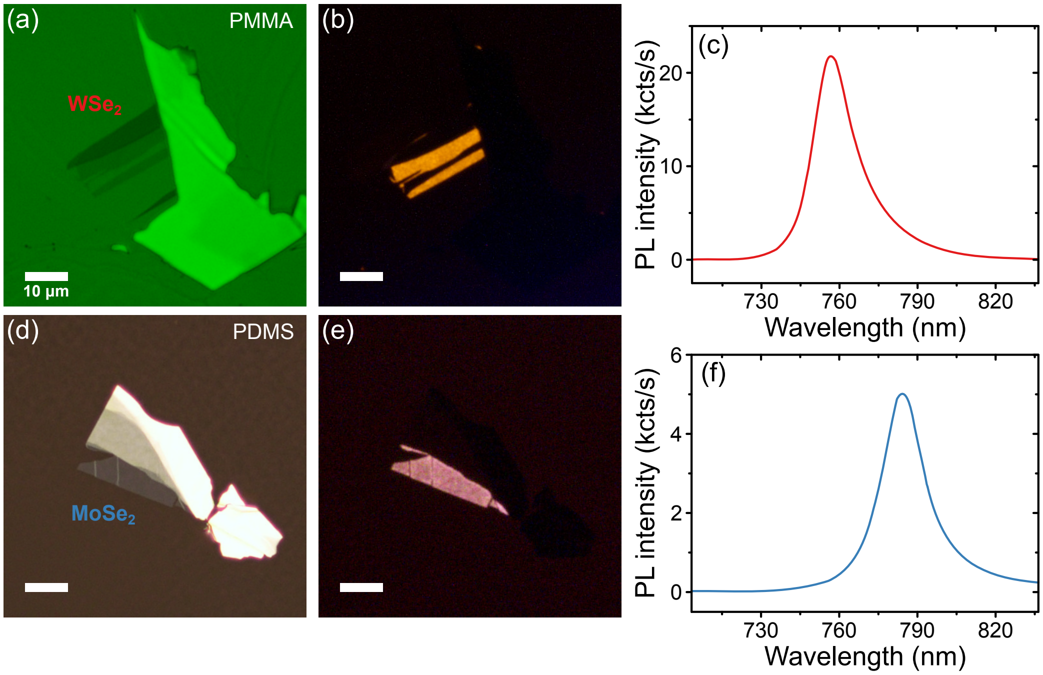


Figure S1: **Optical identification of TMD monolayers on various substrates.** (a) A bright-field image of a $WSe_2$ flake exfoliated onto PMMA-coated $Si/SiO_2$ substrate under green light illumination. (b) A PL image of the sample in(a) acquired using a bright-field microscope. (c) A room temperature PL spectrum recorded in the monolayer region of the sample in (a) using a micro-PL setup. (d) and (e) Bright-field and PL images of a $MoSe_2$ flake exfoliated on a PDMS membrane. (f) A room temperature PL spectrum of the monolayer region of the $MoSe_2$ depicted in (d) and (e).

## Optical identification of TMD monolayers and bilayers on various substrates

The strong dependence of the TMD PL characteristics on the number of atomic layers allows PL imaging to be used for sample thickness identification on various substrates. Figure S1 compares bright-field images of $MoSe_2$ and $WSe_2$ flakes exfoliated onto a PMMA and a PDMS membrane, respectively; green light illumination was used for imaging of the sample on the PMMA membrane in order to make the monolayer region visible.[S1] TMD flakes have very different appearances on these two substrates, with few-layer areas showing neg-


*To whom correspondence should be addressed
†University of Sheffield
‡UNIST
¶University of Oxford
§University of Manchester

ative (positive) optical contrast on PMMA (PDMS). In contrast, monolayer regions of both samples can be easily identified in PL images (Fig. S1 (b) and (e)).

The different colours of $MoSe_2$ and $WSe_2$ in the PL images reflect the difference between their emission spectra. Figure S1 (c) and (f) plots room-temperature PL spectra for the monolayer regions of both flakes recorded using a micro-PL set up. For $MoSe_2$, PL emission arising from exciton recombination is centred at 790 nm while for $WSe_2$ the exciton PL peaks at 750 nm. This difference in the wavelength is readily detected as different colours in the PL images in Figs. S1 (b) and (e).

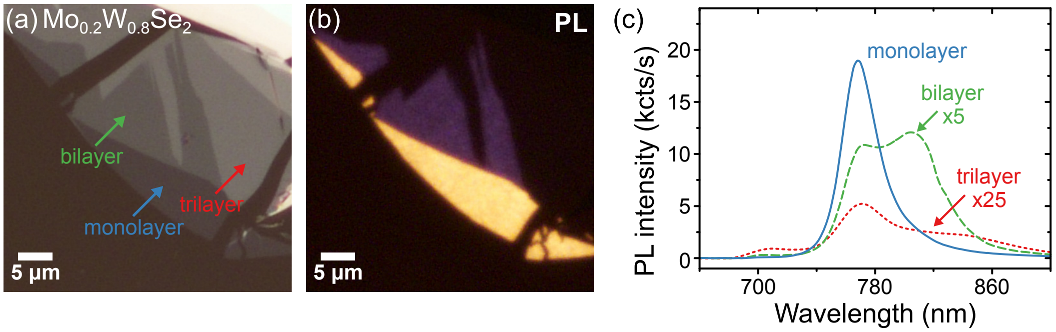


Figure S2: **Photoluminescence imaging of few-layer TMD alloys.** (a) A bright-field image of a few-layer $Mo_{0.2}W_{0.8}Se_2$ flake exfoliated onto a PDMS substrate. (b) A PL image of the sample showing emission from both monolayer and bilayer regions. The variation of the emission colour reflects the difference in the peak PL wavelength as shown in (c). (c) Room-temperature PL spectra recorded in monolayer (blue), bilayer (green) and trilayer (red) regions of the sample.

While PL emission of TMD bilayer has an order of magnitude lower intensity compared to monolayer regions, it can also be detected in PL images. Figure S2 shows bright-field (a) and PL (b) images of a few-layer $Mo_{0.2}W_{0.8}Se_2$ sample exfoliated onto PDMS substrate. Both monolayer and bilayer regions are can be seen in the PL image. The difference in the emission colour and brightness reflects the variation of the PL spectrum with the number of layers. Figure S2 (c) compares room temperature PL spectra recorded in different regions of the flake using a micro-PL set up. The monolayer area shows bright PL centred at 770 nm (blue line), however, the emission peak shifts to longer wavelength and significantly broadens in the bilayer region (dashed green line). The trilayer region (dotted red line) demonstrates

further broadening and reduction of the PL peak, making it invisible in the PL image.

## Selective imaging of different materials in van der Waals heterostructures

The material sensitivity of the PL imaging using a microscope makes it very useful for vdW heterostructure characterisation. Figure S3 shows an optical image of a $MoSe_2$/$WSe_2$ heterostructure assembled on a Si/$SiO_2$ substrate using a viscoelastic stamping method employing PDMS stamps.[S2] The images and PL spectra shown in Fig.S3 are acquired before the structure has been annealed, so weak electronic coupling between the layers is expected. While both TMD crystals have similar appearances in the bright-field microscope image, the PL emission of their monolayer regions has noticeably different colours, allowing the two materials to be easily distinguished.

Selective imaging of different materials within a heterostructure can be further enhanced by replacing the long-pass filter in the detection path of the microscope with an appropriate band-pass filter, as shown in Figure S3 (c) and (d). Here the PL images are recorded using the bandpass filters with the transmission region centred at the emission wavelength of the corresponding material: 750 nm (c) and 790 nm (d), for $MoSe_2$ and $WSe_2$, respectively. As the signal intensity was lowered by the use of a narrow-band filter, 10 s acquisition time was used for both images. Although emission maxima at room temperature for $MoSe_2$ and $WSe_2$ are positioned close to each other, the images demonstrate perfect selectivity, showing only the monolayer region of the chosen material. Figure S3 (e) plots PL spectra recorded in isolated $MoSe_2$ (bottom) and $WSe_2$ (middle) areas, as well as in the overlap region (top). As it is evident from both PL images and spectra, the emission of the heterostructure consists of the sum of $MoSe_2$ and $WSe_2$ emission, indicating a weak coupling between two layers.

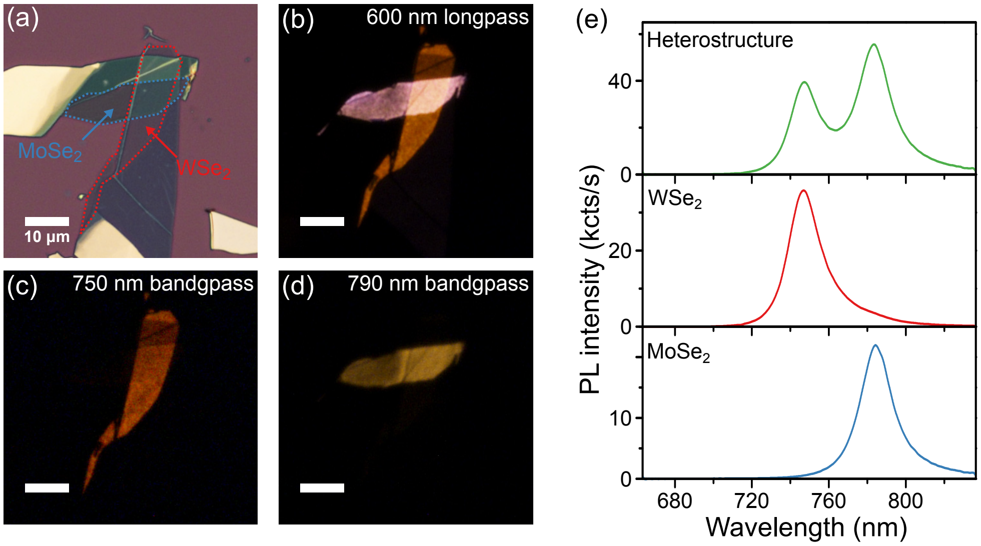


Figure S3: **Selective imaging of different materials in a vdW heterostructure.** All images and PL spectra in this figure are obtained before the sample has been annealed. (a) A bright-field image of a $MoSe_2/WSe_2$ heterostructure assembled on a $Si/SiO_2$ substrate by viscoelastic stamping. (b) A PL image of the sample obtained with a 600 nm long-pass filter showing emission from the monolayer regions of both materials. The overlap region shows PL from both flakes producing another false colour in the image. (c) A PL image of the sample obtained with a 750 nm band-pass filter showing emission from $WSe_2$ monolayer. (d) A PL image of the sample obtained with a 790 nm band-pass filter showing emission from $MoSe_2$ monolayer. (e) PL spectra acquired in the heterostructure (top), isolated $WSe_2$ (middle) and $MoSe_2$ (bottom) regions.

## Quenching of $WS_2$ PL in TMD heterobilayers

The interlayer charge separation in $MoSe_2/WS_2$ heterobilayers leads to significant quenching of the intralayer exciton PL, as shown in Fig. S4. While the reduction of $MoSe_2$ intensity shows strong dependence on the interlayer twist angle (see Fig.5 in the main text), there is no apparent correlation between the $WS_2$ PL and relative rotation of the two layers. Figure S4 compares intralayer $WS_2$ PL spectra collected in the heterobilayer regions with various twist angles.

### CVD growth of $MoSe_2$, $MoS_2$ and $WS_2$

Triangle-shaped $MoSe_2$ monolayers were grown on c-plane sapphire substrates by chemical vapor deposition (CVD). In brief, $MoSe_2$ monolayers were grown by the vaporization of

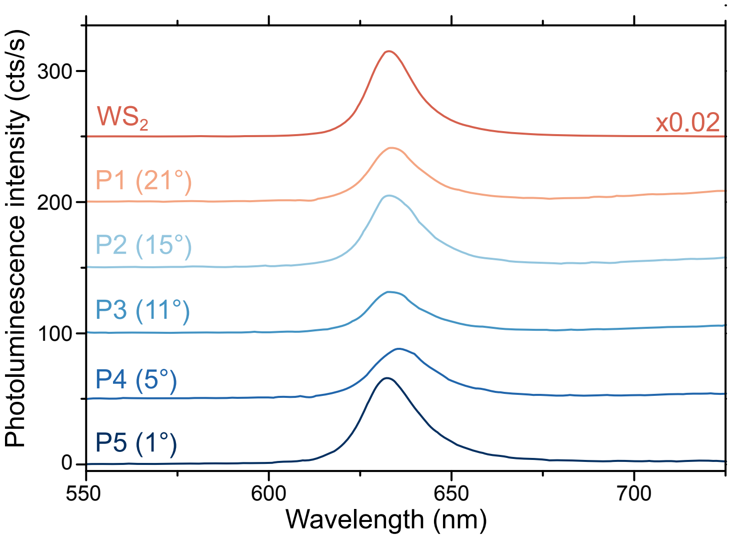


Figure S4: **Quenching of intralayer exciton PL in $WS_2$ within $MoSe_2/WS_2$ heterostructures.** PL spectra for heterostructures assembled from CVD-grown $MoSe_2$ and $WS_2$ monolayers are compared with a CVD-grown $WS_2$ monolayer. The PL spectra are recorded at room temperature in the heterostructure regions shown in Fig.5 of the main text. The same labels, P1-P5, are used here, and correspond to different twist angles (shown in brackets) between the $WS_2$ and $MoSe_2$ monolayers. A spectrum for an isolated $WS_2$ is also shown at the top of the graph. Its as-measured intensity is multiplied by 0.02.

$MoO_3$ and Se powders in a 2-inch quartz tube furnace in a controlled gaseous environment. In a typical run, 60 mg of $MoO_3$ source powder and 100 mg of Se powder were placed in two ceramic boats and loaded into the center heating zone and upwind the low temperature zone in the same quartz tube. A piece of sapphire substrate was placed downstream adjacent to the $MoO_3$ powder as a deposition acceptor. The temperature of $MoO_3$ powder was raised to 600° C at a rate of 25°C/min and then increased 700° C within 10 min. The temperature of the Se powder was raised to 275° C during this 10 min using an external heating coil. The temperature of $MoO_3$ and Se was maintained at 700° C and 275° C, respectively, to facilitate the $MoSe_2$ growth. The vapor-phase reactants were transported by the flowing Ar carrier gas (60 sccm) and selenization was carried out by the flowing $H_2$ reductant gas (12 sccm), thereby facilitating the growth of the 2D $MoSe_2$ crystals at the growth region. After the growth, the furnace was fast cooled to room temperature in an Ar atmosphere only.

For $WS_2$ growth, $WO_3$ powders (50 mg) were loaded at the center of an alumina boat

and then a 300 nm-thick $SiO_2$ substrate was placed upside down above the alumina boat for growth. Another alumina boat containing sulfur powders (200 mg) was placed upstream of the furnace. The furnace was heated to 950°C and maintained for 20 minutes with a flow of Ar gas at 150 sccm in order to grow monolayer $WS_2$. The furnace was then cooled naturally.

For $MoS_2$ growth, a few-drop of Sodium Cholate Hydrate and DI water solution was initially spin-coated on a 300 nm-thick $SiO_2$ substrate and dried at 120°C for solvent evaporation, which acted as a seed layer. Then, this seed layer coated substrate was placed upside down above the alumina boat containing 20 mg of $MoO_3$ powder. Another alumina boat containing sulfur powder (50 mg) was placed upstream of the furnace. The furnace was heated to 750°C at a ramp rate of 20°C/min and maintained for 20 minutes with a flow of Ar gas at 150 sccm in order to grow monolayer $MoS_2$. The pressure inside the chamber was maintained at 400 Torr and finally the furnace was cooled to room temperature naturally.

The as grown monolayer $MoSe_2$ flakes on sapphire substrate were transferred onto a 300 nm $SiO_2$/Si substrate using a PMMA transfer process. Few drops of PMMA (950 K) were spin-coated on the $MoSe_2$/sapphire substrate at 4000 RPM for 60 second. After the spin coating, the sample was dried at 120° C for 30 min. A drop of DI water was put at the interface between PMMA and sapphire, which made the interface wet for easy detachable of PMMA from the sapphire substrate. The piece of PMMA coated $MoSe_2$ was mechanically peeled out from substrate using sharp tweezer and transferred onto DI water. The floating PMMA/$MoSe_2$ was transferred onto a prepared $WS_2$/($SiO_2$/Si) substrate and dried at 80° C for few minute to evaporate the water at the interface. Finally, the PMMA layer was removed using acetone and IPA.

## References

(S1) Blake, P.; Hill, E. W.; Castro Neto, A. H.; Novoselov, K. S.; Jiang, D.; Yang, R.; Booth, T. J.; Geim, A. K. Making graphene visible. *Applied Physics Letters* **2007**, *91*.

(S2) Castellanos-Gomez, A.; Buscema, M.; Molenaar, R.; Singh, V.; Janssen, L.; van der

Zant, H. S. J.; Steele, G. a. Deterministic transfer of two-dimensional materials by all-dry viscoelastic stamping. *2D Materials* **2014**, *1*, 011002.
